# Supplementary material for: Interlayer charge transfer induced by electronic instabilities in the natural van der Waals hetrostructure 4H$_b$-TaS$_2$
Source: arXiv:2411.07823 source file (2024-11-12)
Supplement: Supplementary file 1 [file sm.pdf]

# Supplemental Material for: "Interlayer charge transfer induced by electronic instabilities in the natural van der Waals hetrostructure $4H_b$-$TaS_2$"

R. Mathew Roy,[1] X. Feng,[2] M. Wenzel,[1] V. Hasse,[2] C. Shekhar,[2]
M. G. Vergniory,[2,3] C. Felser,[2] A. V Pronin,[1] and M. Dressel[1]

[1] *1. Physikalisches Institut, Universität Stuttgart, Pfaffenwaldring 57, 70569 Stuttgart, Germany*
[2] *Max Planck Institute for Chemical Physics of Solids, 01187 Dresden, Germany*
[3] *Donostia International Physics Center, P. Manuel de Lardizabal 4, 20018 Donostia-San Sebastian, Spain*

(Dated: November 12, 2024)

## S1. SYNTHESIS

Single crystals of $4H_b$-$TaS_2$ were grown using a chemical vapor transport method from polycrystalline $4H_b$-$TaS_2$ powder, which was synthesized from tantalum and sulfur (Fisher Scientific, Ta: 99.98%, S: 99.9995%). The powder was sealed in an evacuated fused silica ampoule at 600°C for three days. Iodine (3 mg/cm$^3$; Fisher Scientific, 99.999%) was used as the transport additive. The reaction was performed by heating the ampoule in a two-zone furnace with a temperature gradient from 750°C (T2) to 700°C (T1) for several days, after which the ampoule was removed from the furnace and quenched in water. The single crystals were characterized by x-ray powder diffraction.

## S2. EXPERIMENTAL DETAILS

The infrared reflectivity of freshly cleaved crystals of approximately $2 \times 1$ mm$^2$ reflecting-plane size and with the thickness of $\approx 0.5$ mm was measured in the frequency range from 80 cm$^{-1}$ to 20,000 cm$^{-1}$ ( 10 meV to 2.5 eV) as a function of temperature from $T = 325$ to 10 K. We used a Bruker IFS 113v Fourier transform infrared spectrometer for the far-infrared and a Bruker Vertex 80v attached to a Hyperion IR microscope for the mid- and near-infrared ranges, $\omega/(2\pi c) > 650$ cm$^{-1}$. The gold overcoating technique was applied to obtain the absolute reflectivity value for the former and a gold mirror as a reference for the latter method. The complex optical conductivity, $\sigma(\omega) = \sigma_1(\omega) + i\sigma_2(\omega)$, was calculated using the Kramers-Kronig relations with a Hagen-Rubens extrapolations below 80 cm$^{-1}$ and x-ray scattering functions for the high-energy region [1].

## S3. REFLECTIVITY AND OPTICAL CONDUCTIVITY

Fig. S1(a) shows the frequency-dependent reflectivity of $4H_b$-$TaS_2$ for various temperatures as indicated. With decreasing temperature, the low-energy reflectivity rises, indicating a metallic behavior. The dotted lines represent the extrapolated regions obtained using the Hagen-Rubens approximation. Two low-energy absorption features are visible; they appear as peaks in the real part of optical conductivity plotted in Fig. S1(b). The interband contribution to the optical conductivity was calculated by subtracting the fitted Drude term (Fig. S2) from the experimental $\sigma_1$. Any temperature-dependent changes in the interband contribution can be clearly observed in the difference spectra $\Delta\sigma_1$. To observe changes below room temperature, we subtracted the temperature-dependent interband conductivity from 300 K. The temperature evolution of the difference in interband contributions is presented in Fig. S1(c), where $\Delta\sigma_1 = \sigma_1^{\text{interband}}(\omega, T) - \sigma_1^{\text{interband}}(\omega, T = 300\text{ K})$ is plotted. When cooling below 25 K, a clear jump in the hight of the 200-cm$^{-1}$ conductivity peak occurs, indicated by the red ($\leq 20$ K) and blue ($\geq 20$ K) lines. We relate this behavior to the CDW state that occurs in the 1H layer at $T = 24$ K, as discussed in the main text.

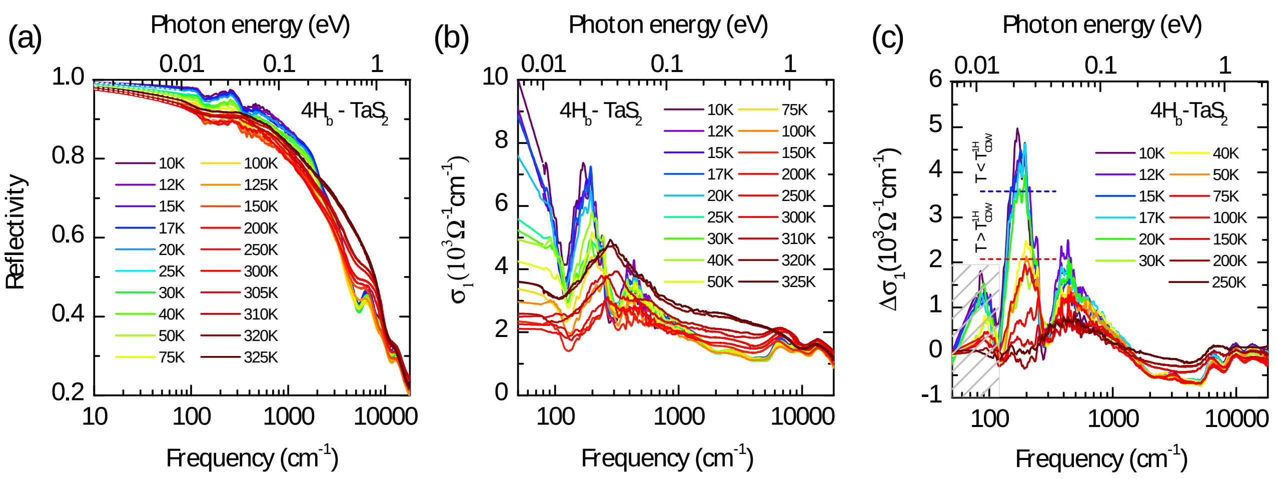


Fig. S1. (a) Temperature evolution of the optical reflectivity of 4H$_b$-TaS$_2$ for all measured temperatures; (b) optical conductivity obtained via Kramers-Kronig analysis; (c) the changes of the interband conductivity compared to the room-temperature behavior (the shaded region at low energies is affected by large uncertainties and is not discussed).

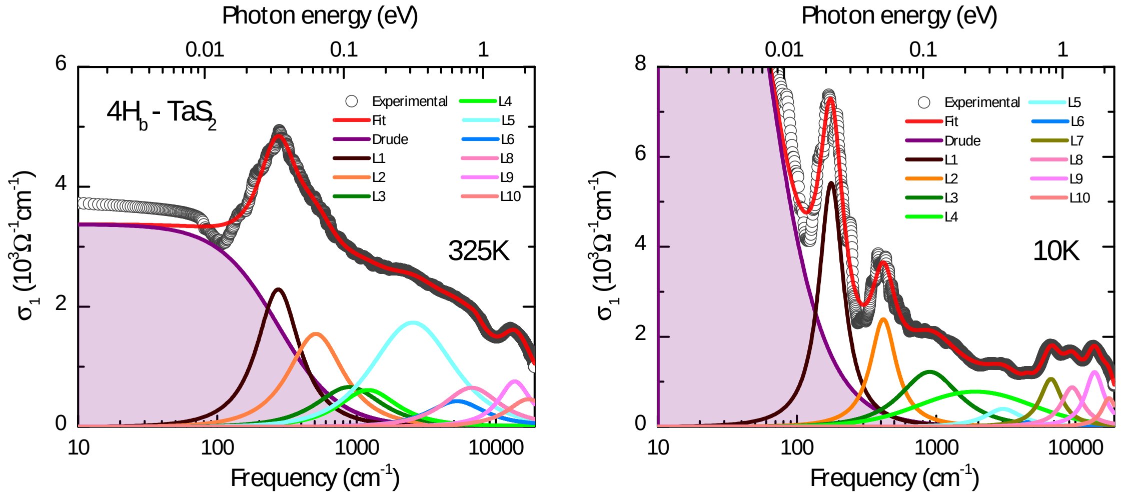


Fig. S2. Examples of the decomposed optical conductivity of 4H$_b$-TaS$_2$ for two temperatures ($T = 325$ K and 10 K), obtained by using the Drude-Lorentz fit procedure.

## S4. DECOMPOSITION OF OPTICAL SPECTRA

The intraband and interband contributions to the total optical conductivity were modeled by adding up the responses of itinerant charges (Drude term) and localized excitations (Lorentz terms):

$$\sigma(\omega) = \sigma_{\text{Drude}}(\omega) + \sigma_{\text{Lorentz}}(\omega) \quad . \tag{1}$$

The complex optical conductivity can also be expressed via the complex dielectric permittivity [$\varepsilon = \varepsilon_1 + \mathrm{i}\varepsilon_2$]:

$$\sigma(\omega) = -i\omega[\varepsilon(\omega) - 1]/4\pi \quad . \tag{2}$$

The Drude-Lorentz approach then becomes:

$$\varepsilon(\omega) = \varepsilon_\infty - \frac{\omega_{p,\text{Drude}}^2}{\omega^2 + i\omega/\tau_{\text{Drude}}} + \sum_j \frac{\Omega_j^2}{\omega_{0,j}^2 - \omega^2 - i\omega\gamma_j} \quad . \tag{3}$$

Here, $\omega_{p,\mathrm{Drude}}$ and $1/\tau_{\mathrm{Drude}}$ are the plasma frequency and the scattering rate of the itinerant carriers, respectively. The parameters $\omega_{0,j}$, $\gamma_j$ and $\Omega_j$ describe the resonance frequency, the width, and the strength of the $j^{th}$ Lorentzian term, respectively.

We have simultaneously fitted $\varepsilon_1$, $\sigma_1$ and the reflectivity by varying the fitting parameters. The decomposition of the optical conductivity is illustrated for two temperatures, $T = 325$ K and 10 K, in Fig. S2. Here, we utilize one Drude and 9 or 10 Lorentzian to fit the experimentally obtained conductivity. The full-width at half-maxima of the Drude peak – the scattering rate $1/\tau$ – decreases with cooling. The Lorentzians L1 and L2 sharpen and move toward lower frequencies at $T \rightarrow 0$. The Lorentzian L7 appears only below $T = 315$ K. The high-frequency Lorentzians sharpen with decreasing temperature; there exists no substantial frequency dependence of their central frequencies.

## S5. FIRST-PRINCIPLES CALCULATIONS

### S5.1. Electronic bands and DOS

First-principles calculations were performed based on the density functional theory (DFT) and density functional perturbation theory (DFPT) implemented in the Vienna ab-initio Simulation Package (VASP) described by the projector augmented wave method [2–5]. The exchange-correlation interaction was included via the generalized gradient approximation (GGA) and parameterized by the Perdew-Burke-Ernzerhof (PBE) functional [6]. The optB86b-vdW method has been adopted for van der Waals (vdW) interactions [7]. The vdW correction was used for the interlayer-distance dependent DOS calculations, see below.

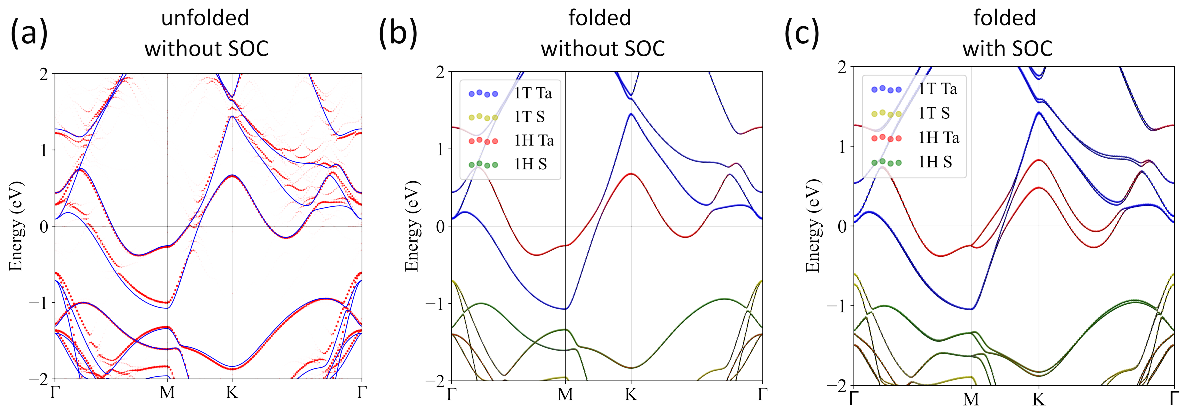


Fig. S3. Band structure of the 1H-1T bilayer system, see details in the text.

The band structure of the 1H-1T bilayer system is shown in Fig. S3: panel (a) is the unfolded band structure with no spin-orbit coupling (SOC), panel (b) is the folded band structure with no SOC, and panel (c) is the folded structure with the SOC included. The bands in Fig. S3 (c) resemble the bulk band structure of $4H_b$-$TaS_2$, making the two-layer calculations a simplified, but reliable approach to theoretically study the DOS-related effects.

Fig. S4 shows the DOS of the 1T layer, 1H layer and the total DOS for two cases: undistorted and after distorting the 1T layer. The calculations were performed for various interlayer distances from 7 Å to 5 Å.

### S5.2. Optical-conductivity calculations

The imaginary part of the interband contribution to permittivity can be obtained from the band structure via:

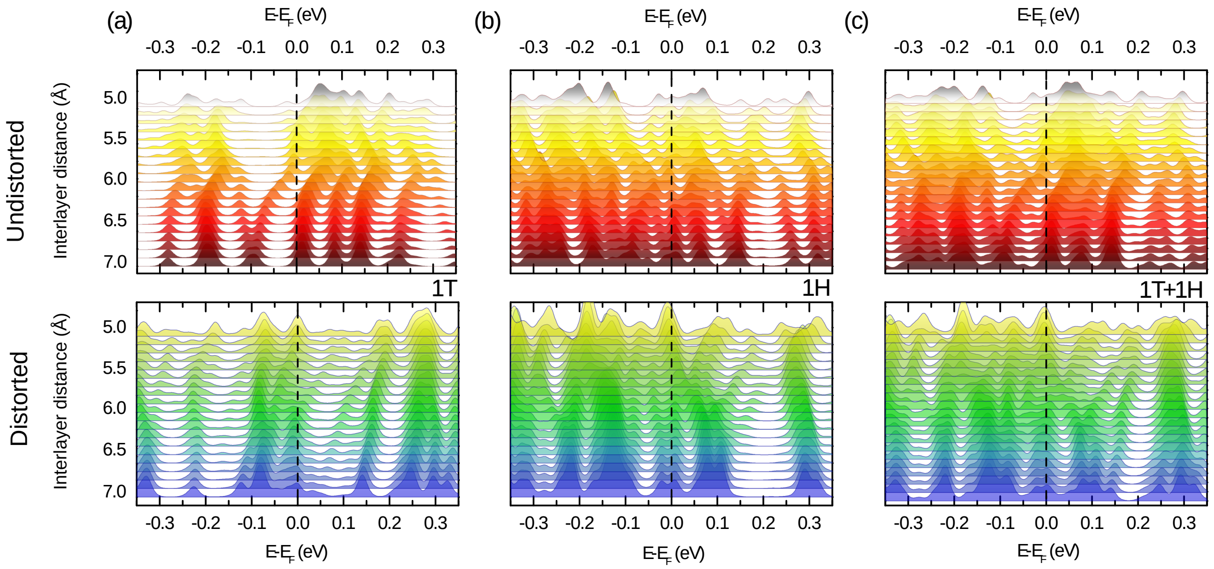


Fig. S4. The interlayer distance-dependent density of states with and without distortion; for the 1T layer (a), for 1H layer (b), and the total density of states (c).

$$\text{Im}\ \varepsilon_{ij}^{\text{inter}}(\omega) = \frac{4\pi^2 e^2}{V} \lim_{q\to 0} \frac{1}{q^2} \sum_{nm;\boldsymbol{k}} 2 f_{n\boldsymbol{k}} \langle u_{m,\boldsymbol{k}+q\boldsymbol{e}_i} | u_{n,\boldsymbol{k}} \rangle \langle u_{n,\boldsymbol{k}} | u_{m,\boldsymbol{k}+q\boldsymbol{e}_j} \rangle \tag{4}$$

$$\times \left[\delta(E_{m,\boldsymbol{k}} - E_{n,\boldsymbol{k}} - \omega) - \delta(E_{m,\boldsymbol{k}} - E_{n,\boldsymbol{k}} + \omega)\right], \tag{5}$$

where $i, j$ is the Cartesian coordinates, $u_{n,\boldsymbol{k}}$ and $E_{n,\boldsymbol{k}}$ denote the band wave function and energy, and $f_{n,\boldsymbol{k}}$ is the Fermi-Dirac distribution function. From here, the real part of permittivity then can be obtained via the Kramers-Kronig relations. The real part of the optical conductivity was calculated via Eq. 2, see Fig. 2(e) of the main text.

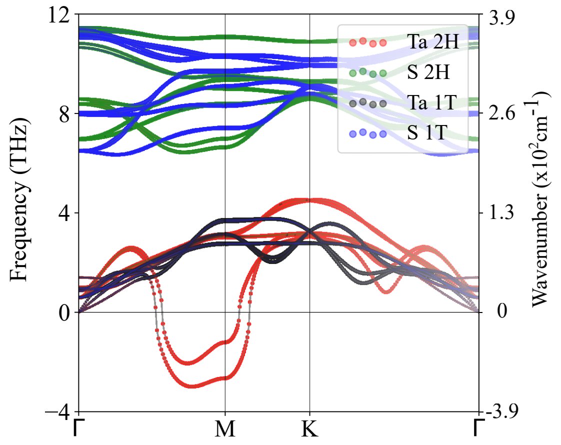


Fig. S5. Phonon dispersion of $4H_b$-$TaS_2$.

### S5.3. Phonons

The phonon spectra were calculated based on 3×3×1 supercells with a Γ-centered 4×4×1 k-mesh with an energy cutoff of 300 eV. Before phonon calculations, the structure was fully relaxed with a force convergence criterion of $10^{-3}$eV/Å. PHONOPY code was used to extract the force constants and phonon spectra [8]. SOC was not included in the phonon calculations. The phonon dispersion in the bulk unit cell of $4H_b$-$TaS_2$ is shown in Fig. S5. There is a phonon instability in the 1H layer. The phonon instability in 1T layer is not visible in the phonon dispersion due to correlation effects in 1T- $TaS_2$.


[1] D. Tanner, Use of x-ray scattering functions in Kramers-Kronig analysis of reflectance, Phys. Rev. B. **91**, 035123 (2015).

[2] G. Kresse and J. Furthmüller, Efficiency of ab-initio total energy calculations for metals and semiconductors using a plane-wave basis set, Comput. Mater. Sci. **6**, 15 (1996).

[3] G. Kresse and J. Furthmüller, Efficient iterative schemes for ab initio total-energy calculations using a plane-wave basis set, Phys. Rev. B **54**, 11169 (1996).

[4] P. E. Blöchl, Projector augmented-wave method, Phys. Rev. B **50**, 17953 (1994).

[5] G. Kresse and D. Joubert, From ultrasoft pseudopotentials to the projector augmented-wave method, Phys. Rev. B **59**, 1758 (1999).

[6] J. P. Perdew, K. Burke, and M. Ernzerhof, Generalized gradient approximation made simple, Phys. Rev. Lett. **77**, 3865 (1996).

[7] J. Klimeš, D. R. Bowler, and A. Michaelides, Van der Waals density functionals applied to solids, Phys. Rev. B **83**, 195131 (2011).

[8] A. Togo and I. Tanaka, First principles phonon calculations in materials science, Scr. Mater. **108**, 1 (2015).
